# Supplementary material for: Instantons and the quantum bound to chaos
Source: arXiv:2212.10202 source file (2023-01-24)
Supplement: Supplementary file 1 [file On_the_statistical_origin_of_the_quantum_bound_to_chaos_PRL_SI.pdf]

On the statistical origin of the quantum bound to chaos -  
Supplementary information

September 2022

# I Methods

## I.1 Quantum calculations

The two-dimensional Hamiltonian described by eq. (8) in the main text was diagonalized on a uniform grid with a Fourier basis, outlined as the discrete variable representation(DVR) in [6]. The eigenvalues and eigenvectors were obtained using the implicitly restarted Lanczos method [11]. The Kubo-regularized OTOC was computed as:

$$\begin{aligned} C_T^{(k)}(t) &= -\frac{1}{\beta\mathcal{Z}} \text{Tr} \left[ \int_0^\beta d\lambda \hat{\rho}_{\beta-\lambda} [\hat{W}(t), \hat{V}(0)]^\dagger \hat{\rho}_\lambda [\hat{W}(t), \hat{V}(0)] \right] \\ &= -\frac{1}{\beta\mathcal{Z}} \sum_{n,m=1}^\infty \int_0^\beta e^{-\lambda E_n} e^{-(\beta-\lambda)E_m} \langle n | [\hat{W}(t), \hat{V}] | m \rangle \langle m | [\hat{W}(t), \hat{V}] | n \rangle \\ &= -\frac{1}{\beta\mathcal{Z}} \sum_{n,m=1}^\infty \frac{e^{-\beta E_n} - e^{-\beta E_m}}{E_n - E_m} |\langle n | [\hat{W}(t), \hat{V}] | m \rangle|^2 \end{aligned}$$

Quantum OTOCs with other regularization procedures can be computed similarly. The Husimi distribution of a density operator  $\hat{\rho}$  can be computed by projecting the operator on a basis of coherent states as:

$$\mathcal{H}_{\hat{\rho}}(\mathbf{p}_0, \mathbf{q}_0) = \langle \mathbf{p}_0, \mathbf{q}_0 | \hat{\rho} | \mathbf{p}_0, \mathbf{q}_0 \rangle \quad (1)$$

where the coherent state  $|\mathbf{p}_0, \mathbf{q}_0\rangle$  is given in the position representation as:

$$\langle \mathbf{q} | \mathbf{p}_0, \mathbf{q}_0 \rangle = \left( \frac{1}{\pi\hbar|\Sigma|} \right)^{1/4} \exp \left\{ -\frac{1}{2\hbar} (\mathbf{q} - \mathbf{q}_0) \Sigma^{-1} (\mathbf{q} - \mathbf{q}_0) + \frac{i}{\hbar} \mathbf{p}_0 \cdot (\mathbf{q} - \mathbf{q}_0) \right\} \quad (2)$$

where the  $\Sigma$  matrix specifies the spread of the coherent state. For a pure state of a 2-dimensional system as in the main text, given by an eigenfunction  $|n\rangle$ , the Husimi section along, say the  $x$ -coordinate (for a fixed  $y_0$ ), can be computed as:

$$\mathcal{H}_n^\pm(x, p_x; y_0) = \langle \mathbf{p}_0, \mathbf{q}_0 | n \rangle \langle n | \mathbf{p}_0, \mathbf{q}_0 \rangle = \langle n | \tilde{\mathbf{p}}, \tilde{\mathbf{q}} \rangle^2 \quad (3)$$

with  $\tilde{\mathbf{p}} = \tilde{\mathbf{p}}(x, p_x; y_0) = \pm 2m(E_n - V(x, y_0) - p_x^2/2m)$  and  $\tilde{\mathbf{q}} = (x, y_0)$ .

## I.2 Ring-polymer propagation

The ring-polymers described in the main text were sampled and propagated in real time using suitable symplectic integrators. A basic symplectic verlet integrator up-

dates the position and momenta for one time-step as:

$$\begin{aligned}\mathbf{p}_k &= \mathbf{p}_{k-1} + b_k \mathbf{F}_{k-1} & \dots \text{ B} \\ \mathbf{q}_k &= \mathbf{q}_{k-1} + a_k \frac{\mathbf{p}_k}{m} & \dots \text{ A}\end{aligned}$$

for  $k = 1, 2 \dots n$ . Here,  $F_k$  is the force computed at the system configuration specified by  $\mathbf{q}_k$  and  $a_k, b_k$  are coefficients that depend on the order  $n$  of the integrator. For  $n = 2$ ,  $a_1 = 1.0, a_2 = 0.0, b_1 = b_2 = 0.5$ , which corresponds to the velocity verlet integrator.

A thermal distribution of ring polymers can be efficiently obtained from the velocity verlet algorithm by combining it with a *path-integral Langevin equation* thermostat (PILE) [4]. This effectively involves adding an additional momentum update step given as:

$$\mathbf{p}_k = c_k^{(1)} \mathbf{p}_k + c_k^{(2)} \boldsymbol{\xi}_k \quad \dots \text{ O}$$

(where  $c_k^{(1)}$  and  $c_k^{(2)}$  are coefficients that depend on the temperature and mass and  $\boldsymbol{\xi}_k$  is a Gaussian random number) to the A and B steps above. For computing the thermal OTOCs in fig. (2) in the main text, the system was thermalized for 50 atomic units of time (obtained by setting  $\hbar = 1.0$  and  $k_B = 1.0$ ) with a timestep  $dt = 0.05 \text{ a.u.}$

The monodromy matrix, which is required for calculating classical and RPMD OTOC, can be propagated using a fourth order symplectic integrator as detailed in [3]. This algorithm updates the monodromy elements as follows:

$$\begin{aligned}\mathbf{M}_{pp}^{(k)} &= \mathbf{M}_{pp}^{(k-1)} - b_k \mathbf{H}_k \mathbf{M}_{qp}^{(k-1)} & \dots \text{ M1} \\ \mathbf{M}_{pq}^{(k)} &= \mathbf{M}_{pq}^{(k-1)} - b_k \mathbf{H}_k \mathbf{M}_{qq}^{(k-1)} & \dots \text{ M2} \\ \mathbf{M}_{qp}^{(k)} &= \mathbf{M}_{qp}^{(k-1)} + a_k \frac{\mathbf{M}_{pp}^{(k-1)}}{m} & \dots \text{ M3} \\ \mathbf{M}_{qq}^{(k)} &= \mathbf{M}_{qq}^{(k-1)} + a_k \frac{\mathbf{M}_{pq}^{(k-1)}}{m} & \dots \text{ M4}\end{aligned}$$

where  $\mathbf{H}_k$  is the Hessian matrix of the system for the system configuration specified by  $\mathbf{q}_k$ .

### I.3 Computing ring-polymer Lyapunov exponents

The Lyapunov exponents in fig. (2b) in the main text were also computed using symplectic integrators by propagating the *tangent dynamics* [16] of the system in

parallel to the above dynamical variables. The tangent dynamics Hamiltonian is given in terms of the tangent variables  $\delta\mathbf{q}$  and  $\delta\mathbf{p}$  as follows:

$$H(\delta\mathbf{p}, \delta\mathbf{q}; t) = \frac{\delta\mathbf{p} \cdot \delta\mathbf{p}}{2m} + \frac{1}{2} \delta\mathbf{q}^T \mathbf{D}_V^2(\mathbf{q}_t) \delta\mathbf{q} \quad (4)$$

where  $\mathbf{D}_V^2(\mathbf{q}_t)$  is the Hessian of the system at time  $t$ . The dynamics of this tangent dynamics Hamiltonian can be simultaneously computed using the symplectic integration schemes in the previous section with the following additional steps:

$$\delta\mathbf{p}_k = \delta\mathbf{p}_{k-1} + b_k \mathbf{H}_{k-1} \delta\mathbf{q}_{k-1} \quad \dots B_v \quad (5)$$

$$\delta\mathbf{q}_k = \delta\mathbf{q}_{k-1} + a_k \frac{\delta\mathbf{p}_k}{m} \quad \dots A_v \quad (6)$$

Since the RPMD OTOCs are computed from dynamics of the centroid (in the force field generated by the potential energy and ring-polymer fluctuations), the relevant maximal characteristic Lyapunov exponent is that of the ring-polymer centroid which is obtained as:

$$\lambda_{mCE}(\mathbf{Q}_0, \mathbf{P}_0) = \lim_{t \rightarrow \infty} \frac{1}{t} \ln \frac{\|W_0(t)\|}{\|W_0(0)\|} \quad (7)$$

where  $\|W_0(t)\|^2 = \|\delta\mathbf{P}_0(t)\|^2 + \|\delta\mathbf{Q}_0(t)\|^2$ . Here, the centroid tangent momentum and position are initialized with small values  $|\delta\mathbf{P}_0| = \epsilon_1, |\delta\mathbf{Q}_0| = \epsilon_2$ . The Lyapunov exponents varies across the phase space, so we compute the exponent from phase space saddle points which channels the dynamics between the two wells. We obtained the maximal exponent from collapsed ring polymers above  $T_c$  (which corresponds to the classical saddle), and from ring-polymer instantons below  $T_c$ . The ring-polymer instantons were found using an eigenvector following technique that finds saddle points in the ring-polymer potential energy surface [13, 5, 14].

#### I.4 Classical and ring-polymer Poincaré section

The classical Poincaré surface of section(PSOS) at an energy  $E$  is obtained as follows: phase space trajectories are initialized with random momenta various points in the configuration space such that the total energy  $\frac{\mathbf{p}^2}{2m} + V(\mathbf{q}) = E$ . The system is ‘relaxed’ for 50 a.u. of time, after which Poincare sections are computed with trajectories whose length ranges from 200-100 a.u. of time. All classical PSOSs are computed with  $y_0 = 0.0$  and  $p_y > 0$  to visualize the dynamics around the saddle point.

For computing ring-polymer sections and the respective ‘microcanonical’ OTOCs, collapsed ring-polymers were initialized at all regions in phase space with a total

energy  $NE$  ( $N$  is the number of beads) and allowed to relax for about 100 a.u. of time. The microcanonical OTOCs were obtained by propagating the monodromy matrices of the resultant ring-polymer configurations. The centroid PSOS is plotted by recording the  $X_0$  and  $P_{X,0}$  (the centroid  $x$ -coordinate and momenta) whenever the ring-polymer crosses the hyperplane  $Y_0 = 0$  with  $P_{Y,0} > 0.0$ . The phase-space of the ring-polymer is  $2Nd$ -dimensional for a  $d$ -dimensional system, so the constant energy hypersurface has a dimension  $2Nd - 1$ . So, the centroid PSOS is just a convenient 2-dimensional projection of this hypersurface and is not quite the same as the classical PSOS.

### I.5 Histograms of $r_g$ distribution

The radius-of-gyration  $r_g$  of the ring polymer computed w.r.t the centroid as:

$$r_g = \left| \frac{\sum_{i=1}^N \|\mathbf{q}_i - \mathbf{Q}_0\|^2}{N} \right|^{1/2} \quad (8)$$

indicates its degree of delocalization. The  $r_g$  values fluctuate in general along a ring-polymer trajectory, however, the fluctuations are minimal for integrable trajectories. We hence computed the maximal  $r_g$  over ring-polymer trajectories of length 1000 a.u and plotted a histogram of the resultant max  $r_g$  distribution. Below the cross-over temperature  $T_c$ , we found the histogram to be bimodal, indicating ‘instantonization’ of ring-polymer phase space.

## II Scrambling pathways and state-mixing

It is a well-known conjecture that most eigenstates of a quantum system with a mixed classical phase space are either localized in the regular islands or on the chaotic sea [15]. One of the important findings of our work is that quantum scrambling pathways which contribute to exponential growth are precisely between such quantum states that are localized in a region of stability and those localized in a region of instability (characterized by the eigenvalues of the Hessian). In figure 1, we show two low-energy quantum states and all possible scrambling pathways  $b_{nm}$  between them. It is clearly evident that the only exponential contribution is between  $n = 1$  (localized in the wells) and  $n = 3$  (localized on the phase-space saddle point). The corresponding quantum wavefunctions, however show no imprints of the underlying classical dynamics.

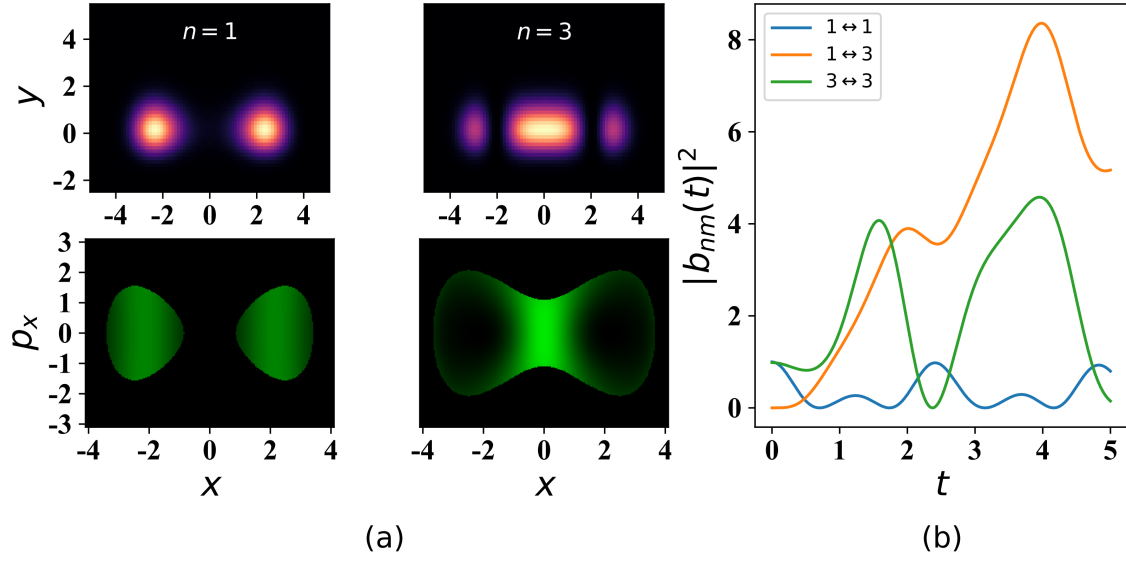

Figure 1: (a) Quantum wavefunctions and Husimi sections for the 2D coupled double well described in the main text which localize inside the well (left) and at the (phase-space) saddle point respectively. (b) Contributions from different possible scrambling events  $b_{nm}$  between states in (a).

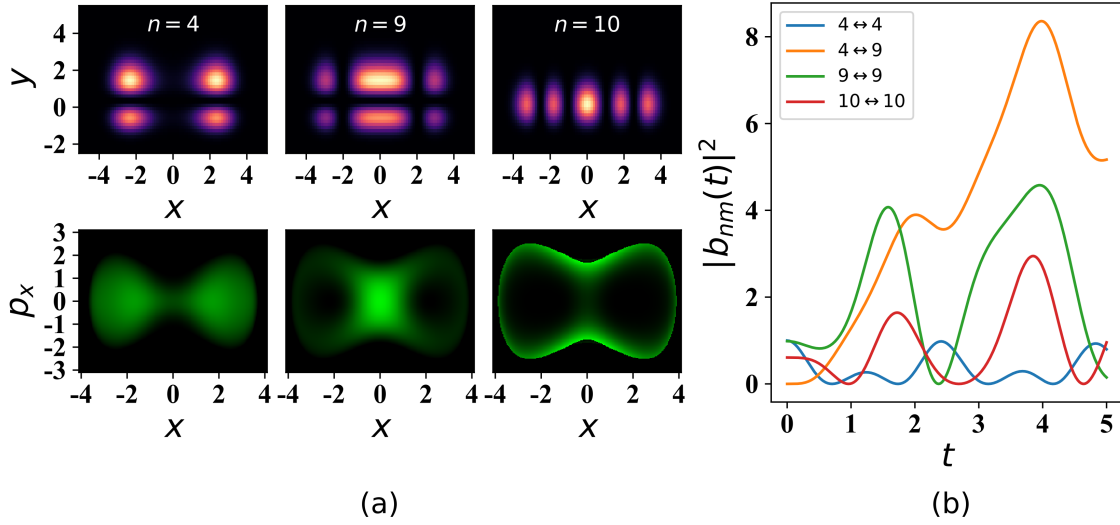

Figure 2: Same as in fig. 1 but with different quantum states for the uncoupled case ( $z = 0.0$ ). Exponential growth of  $b_{nm}$  is again between states which differ in the instability of the region they localize.

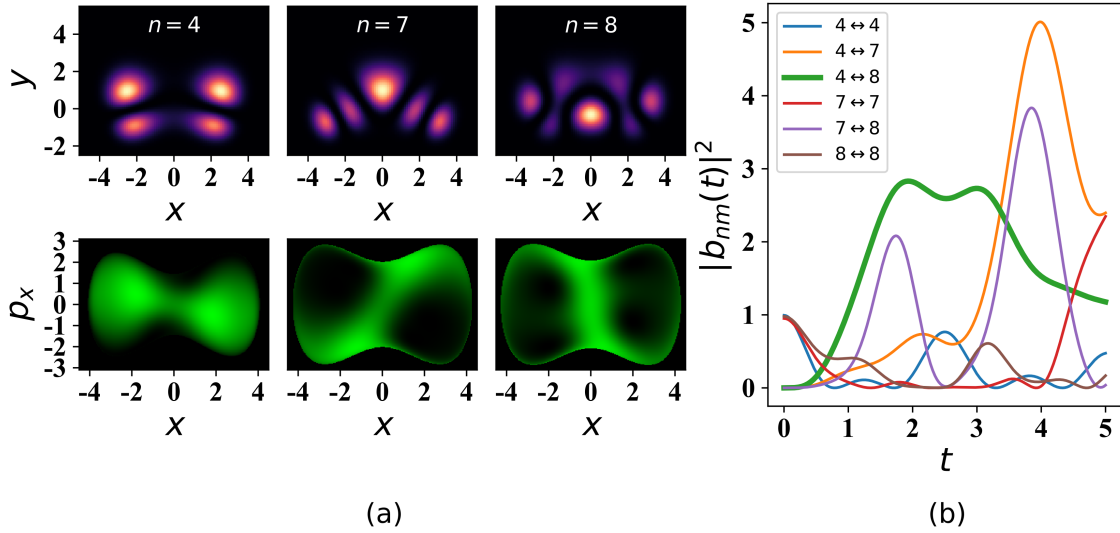

Figure 3: (a) Same as in fig. 2 but for the coupled double well ( $z = 1.0$ ). The wavefunctions and Husimi sections clearly indicate state mixing, which alters the scrambling pathways. (b) The dominant (exponential) scrambling pathway in fig. 2 is altered by perturbations and is plotted in green.

In figure 2, we show the wavefunctions and Husimi sections of a few higher-energy eigenstates for the uncoupled ( $z = 0.0$ ) PES in the main text. The system is non-chaotic and the eigenstates can be clearly assigned w.r.t. the composite one-dimensional systems. For instance, the  $n = 9$  state is formed from the one-dimensional wavefunctions with  $n_x = 3, n_y = 2$ , and  $n = 10$  from  $n_x = 5, n_y = 1$ . The Husimi sections indicate that they localize on the phase-space saddle point and a resonant classical trajectory respectively.

However, switching on perturbations ( $z \neq 0$ ) prevents such a clear eigenstate assignment in general. In fig. 3, the  $n = 7, 8$  are perturbed eigenfunctions originating from  $n = 8, 9$  of the uncoupled case respectively. The Husimi sections indicate that they are no longer ‘pure’, i.e. they are now localized on both the saddle point and the resonant trajectory. The plots of  $b_{nm}$  once again indicate that exponential scrambling is between states localized in the wells ( $n = 4$ ) and those localized on the saddle-point ( $n = 7, 8$ ).

For high-energy eigenstates, the level-spacing statistics follows the Wigner-Dyson distribution, in line with the *Bohigas-Giannoni-Schmit (BGS)* conjecture[2, 1]. However, since these states only become accessible when the system has high thermal energy, we expect that the corresponding quantum thermal OTOC to be well approx-

imated by classical dynamics and statistics. The MSS bound is hence relevant when the system's dynamics is affected by a few low-energy eigenstates.

### III Comparison of different regularization

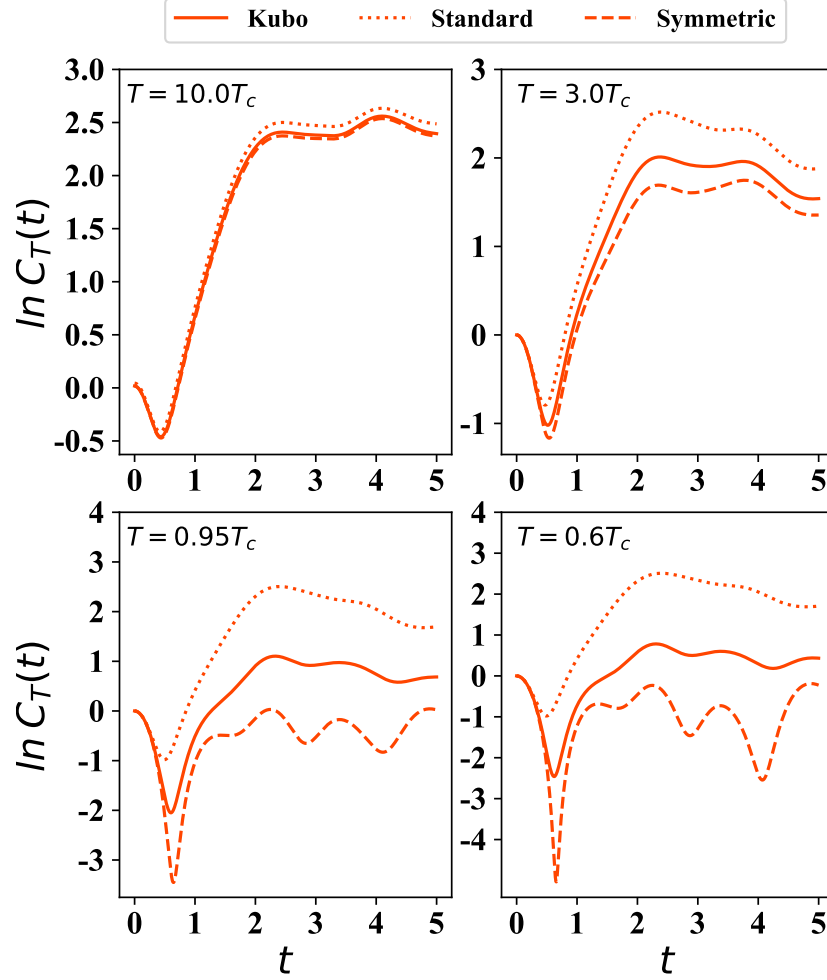

Figure 4: Comparison between the thermal OTOCs at four temperatures obtained from three different regularization procedures.

The quantum thermal OTOCs can be computed as mentioned in the main text:

$$C_T^{(\cdot)}(t) = \sum_{n,m=1}^{\infty} P_{nm}^{(\cdot)} |b_{nm}(t)|^2 \quad (9)$$

with

$$P_{nm}^{(u)} = \frac{1}{\mathcal{Z}} e^{-\beta E_n} \quad P_{nm}^{(s)} = \frac{1}{\mathcal{Z}} e^{-\beta(E_n + E_m)/2} \quad P_{nm}^{(k)} = \frac{1}{\beta \mathcal{Z}} \frac{e^{-\beta E_n} - e^{-\beta E_m}}{E_m - E_n} \quad (10)$$

At high temperatures ( $\beta \ll 1$ ), the structure of the thermal OTOCs do not differ much w.r.t the regularization (see fig. 4). At lower temperatures, the unregularized thermal OTOC grows at a faster rate and below  $T_c$ , it continues to grow at the ‘classical’ growth rate, and violates the MSS bound. The Kubo-regularized thermal OTOC still grows exponentially at  $T \sim T_c$ , while the symmetrized OTOC ceases to be exponential. The unregularized OTOC continues to grow exponentially much below  $T_c$  ( $0.6T_c$ ), thereby violating the bound. Semiclassically, we can attribute this to the inclusion of non-centroid thermal fluctuations. The Kubo-regularized and symmetrized OTOCs satisfy the bound at all temperatures considered.

## IV Choice of system parameters

All simulations in the main text use the following system parameters:  $\lambda = 2.0, g = 0.08, \alpha = 0.382, D = 3V_b = 9.375$ . The system size is decided by the parameter  $g$  and [8] sets  $g = 0.02$ , which makes the system ‘classical’ with no exponential thermal OTOC at  $T \sim T_c$ . For  $g = 0.08$  and  $\alpha = 0.382$ , the component one-dimensional systems have 2 quantum states below the barrier energy  $V_b = \lambda^4/64g$ , which is required for converging the RPMD OTOCs w.r.t. the number of bead replicas. Moreover, classical chaos in the de Leon-Berne potential exhibits an interesting non-monotonic dependence w.r.t to the  $\alpha$  parameter, which is related to the ‘coupling frequency’  $\omega_m = (2D\alpha^2/m)^{1/2}$  of the Morse potential with the one-dimensional double well.

In fig. 5, the wavefunctions, classical PSOS and Husimi sections for the states (that have state mixing) which correspond to  $n_x = 3, n_y = 2$  in the uncoupled case are plotted for different  $\alpha$  values. They vary in the number of Morse eigenstates with energy less than  $V_b$ . As is evident from fig. 5, the phase space volume of chaotic trajectories varies non-monotonically with  $\alpha$ . We expect this  $\alpha$ -dependence to be related to underlying classical resonances. For the value  $\alpha = 0.382$  used in the main text, classical chaos imprints itself onto the quantum dynamics in the form of eigenstate mixing, which is evident from the Husimi section.

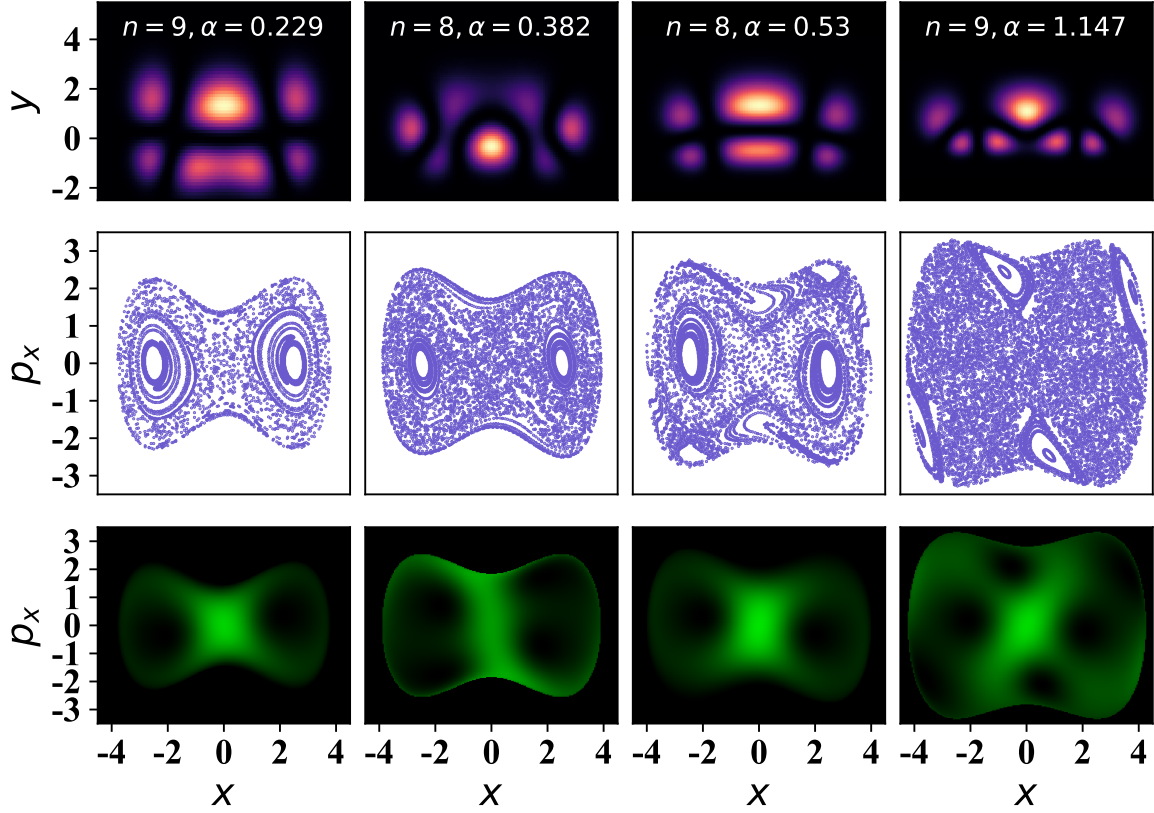

Figure 5: Plots of the wavefunction and the classical Poincaré sections and quantum Husimi sections at the respective energies for different values of  $\alpha$ . The non-monotonicity in the degree of chaos is evident from the difference in the regions of integrability as  $\alpha$  varies. These changes manifest as varying degrees of state-mixing in the respective Husimi sections.

## V Thermal OTOCs and real-time quantum coherence

Since the two-dimensional double-well system has a small system size (governed by the parameter  $g$ ), real time coherence effects are prevalent in the short-time dynamics of the system, due to interference between forward and backward Feynman paths. As mentioned in [12], the ‘dissipation’ time or ‘decoherence’ time  $t_d$  is also of relevance in chaotic systems, and it had been identified as the timescale at which two-point thermal correlators of the form  $\langle \hat{V}(0)\hat{W}(t) \rangle_\beta$  decay exponentially. In fig. 6, we plot the Kubo-regularized position auto-correlation function along the  $x$ -coordinate for the coupled and uncoupled double well at  $T = 0.95T_c$ . The time period of the oscillations ( $\sim 150$  a.u.) correspond to a frequency of  $\sim 0.042$  Hartree  $\hbar^{-1}$ , which corresponds precisely to the tunneling splitting energy between the first-two quantum states of

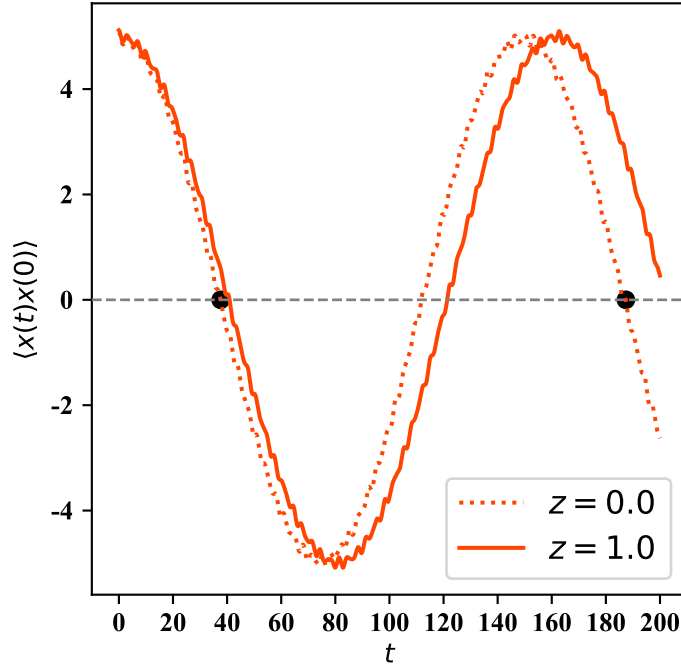

Figure 6: The x-coordinate of the (Kubo-regularized) position auto-correlation functions for the coupled and uncoupled double well potential in the main text, at  $T = 0.95T_c$ .

the one-dimensional component double well. This clearly indicates that the main source of real-time coherence in the double-well system that this article is concerned with, is from deep tunneling under the barrier. The coherence effects are slightly minimized by the transverse coupling with a Morse potential, as indicated by the decreased frequency of oscillations when  $z = 1.0$ , however they are not eliminated.

Exponential scrambling, as indicated by a thermal OTOC, however is expected to begin after the decoherence time  $t_d$ . In fig. 7, we plot the position-momentum correlators at the three different temperatures considered in the main text (The scrambling events  $b_{nm}$  are obtained from the difference in the contributions from the two possible operator orderings of these correlators). The RPMD and quantum correlators are in quantitative agreement until about  $0.7 \text{ a.u.}$ , the time after which exponential scrambling begins. This clearly indicates that real-time coherence effects occur concomitantly with exponential scrambling in this system.

The effect of real-time coherence on thermal OTOCs can be understood from the ‘microcanonical’ contributions to scrambling at a given temperature. The quantum

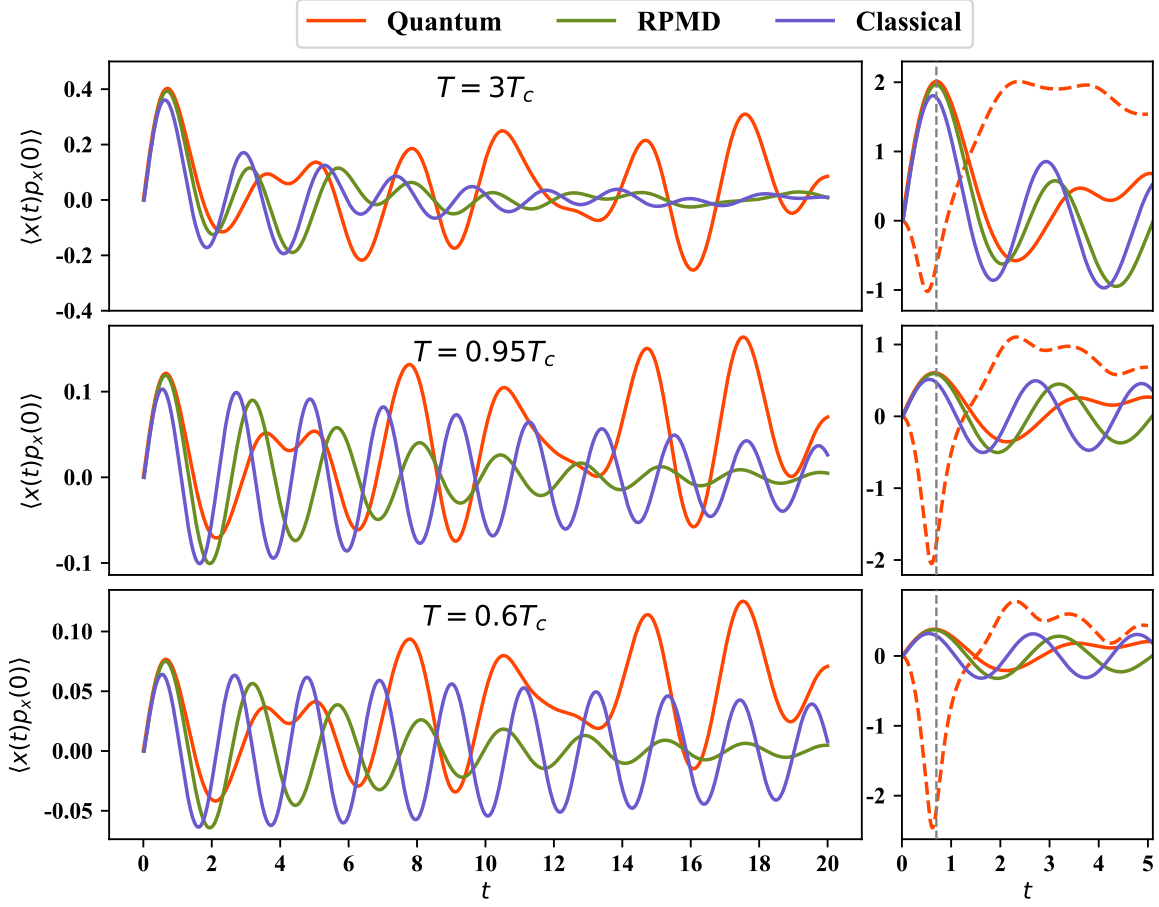

Figure 7: (a) Plots of the position-momenta thermal correlator at 3 temperatures. (b) Same as in (a), but with the correlators amplified 5 times for comparison with the quantum thermal OTOC (orange dashed line). The grey vertical lines indicate the time until which RPMD and quantum OTOCs are in quantitative agreement.

microcanonical OTOCs can be computed as in [8]:

$$c_n(t) = -\langle n | [x(t), p_x(0)]^2 | n \rangle \quad (11)$$

And, the classical and RPMD microcanonical contributions to the corresponding semiclassical OTOCs can be computed as in the main text:

$$C_{mc}^N(t) = \int_{E=NV_b} d\tilde{\mathbf{P}} d\tilde{\mathbf{Q}} \left| \frac{\partial X_0(t)}{\partial X_0} \right|^2 \quad (12)$$

The plots of the above quantities are provided in fig. 8 for the component one-dimensional double well. Exponential growth of the classical microcanonical OTOC necessitates the presence of points in the configuration space with a negative Hessian

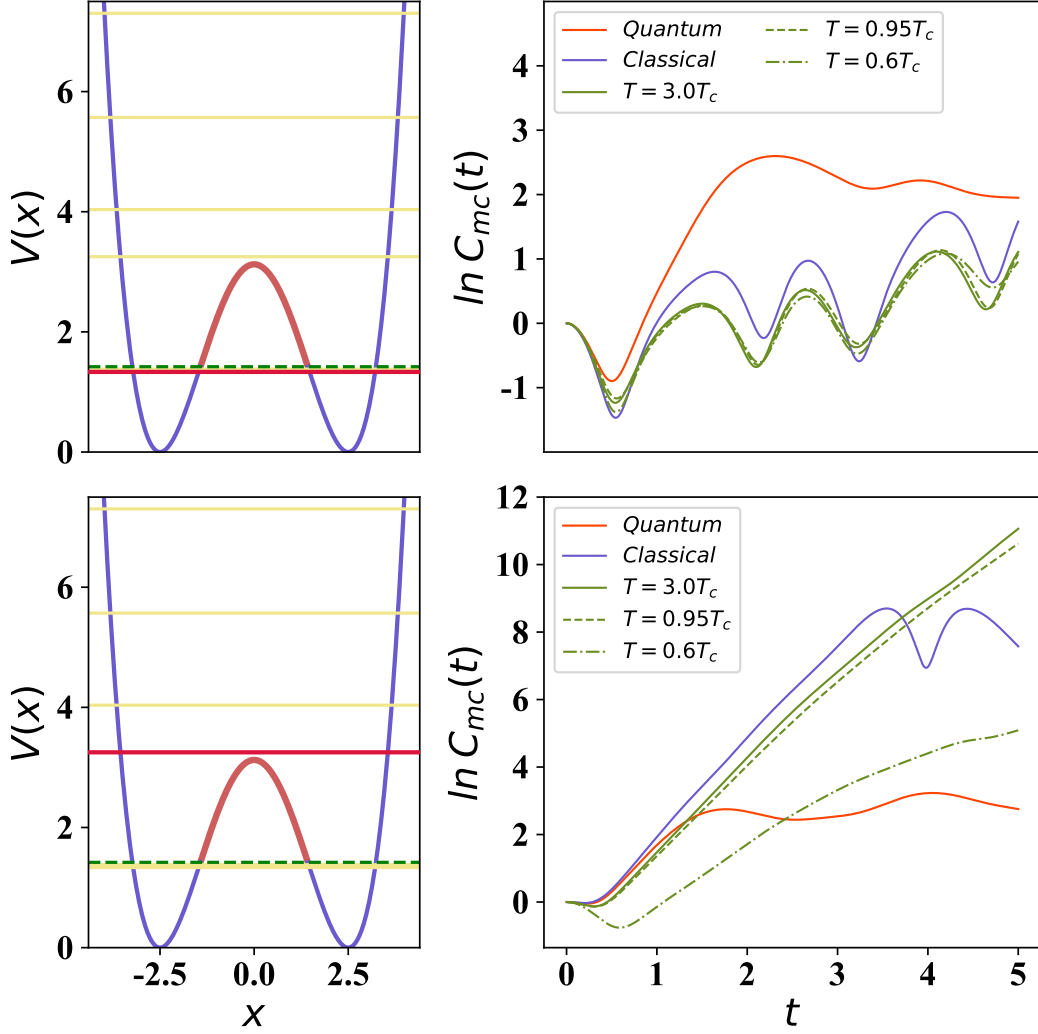

Figure 8: (a) Eigen state energies of the double well (light green). The green dashed line indicates the point at which the Hessian changes sign. The classical microcanonical OTOC can grow exponentially in the region marked in red. (b) The quantum, classical and RPMD microcanonical OTOC at the energy marked by the horizontal crimson line in (a).

eigen value at the given energy, whereas quantum microcanonical OTOC can grow exponentially regardless of that, due to coherent tunneling. In fig. 8, at  $E = 1.3$ , the semiclassical OTOCs are sinusoidal whereas the quantum OTOC is exponential, clearly indicating scrambling ‘under’ the barrier by coherent tunneling. For  $E = 3.18 \sim V_b$ , all the OTOCs are exponential; RPMD OTOC has a temperature-dependent exponent indicating temperature-dependent instanton tunneling. This explains the discrepancy (of about  $0.14 \text{ a.u.}^{-1}$ ) between the quantum and RPMD ther-

mal OTOC growth rate  $T = 0.95T_c$  in the main text, as imaginary-time path-integral based methods explicitly neglect real-time coherence [9]. While a quantitative agreement between the RPMD OTOC growth rate and scrambling timescale is prevented by real-time coherence effects, our results strongly suggests that the bound on chaos proposed by [12] has its origin in thermally-assisted (generalized) instanton tunneling, as they contribute majorly to exponential growth.

For the ‘classical’ parameters considered by [8], there are no energies where the quantum microcanonical OTOCs are exponential, while the semiclassical OTOCs are sinusoidal (figure not shown). This clearly indicates that the effects of real-time coherence are minimal on the quantum OTOC and also explains why there is no exponential scrambling at  $T \sim T_c$  for those parameters. It is also evident that it is in this regime - where scrambling is marred by real-time coherence, where the bound in [12] is relevant, at least for low-dimensional systems with small size. In the absence of a discernible barrier in the configuration, real-time coherent effects can be expected to manifest as *dynamical tunneling* [7, 10].

## VI Growth rate of thermal OTOCs

It has been pointed out [8, 17] that a ‘naive’ semiclassical approximation of the thermal OTOC will predict its growth rate at very high temperature as:

$$C_T(t) \sim \hbar^2 e^{2\lambda_{cl}t} \quad (13)$$

where  $\lambda_L = \lambda$  is the classical Lyapunov exponent (corresponding to the saddle point), whereas

$$C_T(t) \sim e^{\lambda t} \quad (14)$$

at all temperatures considered for the system in the main text. We provide an explanation to the halving of the growth rate when the trajectories are Boltzmann-weighted. The following factorization holds for the classical stability matrix elements:

$$\frac{\partial x_t}{\partial p_{x,0}} = \mathcal{S}(t; \mathbf{p}, \mathbf{q}) \exp(\Lambda(t; \mathbf{p}, \mathbf{q})) \quad (15)$$

where  $\mathbf{q}, \mathbf{p}$  are the initial momenta and position respectively. Here,  $|\mathcal{S}(t; \mathbf{p}, \mathbf{q})| \leq 1$  and  $\Lambda(t; \mathbf{p}, \mathbf{q}) \geq 0$ , i.e. the stability matrix elements are either sinusoidal or exponen-

tial or a product of the two. We then have:

$$C_T^{(cl)}(t) = \frac{1}{\mathcal{Z}_{cl}} \int d\mathbf{p} d\mathbf{q} e^{-\beta H(\mathbf{p}, \mathbf{q})} \left| \frac{\partial x_t}{\partial p_{x,0}} \right|^2 \leq e^{\lambda t} \int d\mathbf{p} d\mathbf{q} e^{-\beta H(\mathbf{p}, \mathbf{q})} \mathcal{S}(t; \mathbf{p}, \mathbf{q}) \frac{\partial x_t}{\partial p_{x,0}} \quad (16)$$

as  $\lambda$  is the maximal Lyapunov exponent for the system. Integrating the RHS above by parts, we obtain:

$$C_T^{(cl)}(t) \leq e^{\lambda t} \int d\mathbf{p} d\mathbf{q} e^{-\beta H(\mathbf{p}, \mathbf{q})} x(t) \frac{\partial \mathcal{S}(t; \mathbf{p}, \mathbf{q})}{\partial p_{x,0}} \quad (17)$$

Since the function  $e^{-\beta H}$  is positive, by the Cauchy Schwartz inequality of weighted inner products, we get:

$$C_T^{(cl)}(t) \leq e^{\lambda t} (\langle x(t)^2 \rangle_\beta)^{1/2} \left( \left\langle \left( \frac{\partial \mathcal{S}}{\partial p_{x,0}} \right)^2 \right\rangle_\beta \right)^{1/2} \quad (18)$$

where  $\langle A \rangle_\beta = \int \int d\mathbf{p} d\mathbf{q} e^{-\beta H} A$ . Since the thermal expectation values of operators are bounded,

$$C_T^{(cl)}(t) = O(e^{\lambda t}) \quad (19)$$

provided  $\frac{\partial \mathcal{S}(t)}{\partial p_{x,0}}$  has, at most, a polynomial growth rate. Since  $\mathcal{S}(t)$  is trigonometric by definition, we can expect this indeed to be the case. This argument holds for the matrix elements  $M_{qq}$  considered in the main text (The choice of  $M_{pq}$  for the derivation above is purely for convenience). So, above  $T_c$ , the classical OTOC ‘trivially’ satisfies the bound.

# Bibliography

- [1] O Bohigas, MJ Giannoni, and C Schmit. “Spectral properties of the Laplacian and random matrix theories”. In: *Journal de Physique Lettres* 45.21 (1984), pp. 1015–1022.
- [2] O. Bohigas, M. J. Giannoni, and C. Schmit. “Characterization of Chaotic Quantum Spectra and Universality of Level Fluctuation Laws”. In: *Phys. Rev. Lett.* 52 (1 Jan. 1984), pp. 1–4. DOI: [10.1103/PhysRevLett.52.1](https://link.aps.org/doi/10.1103/PhysRevLett.52.1). URL: <https://link.aps.org/doi/10.1103/PhysRevLett.52.1>.
- [3] Mark L Brewer, Jeremy S Hulme, and David E Manolopoulos. “Semiclassical dynamics in up to 15 coupled vibrational degrees of freedom”. In: *The Journal of chemical physics* 106.12 (1997), pp. 4832–4839.
- [4] Michele Ceriotti et al. “Efficient stochastic thermostating of path integral molecular dynamics”. In: *The Journal of chemical physics* 133.12 (2010), p. 124104.
- [5] Charles J Cerjan and William H Miller. “On finding transition states”. In: *The Journal of chemical physics* 75.6 (1981), pp. 2800–2806.
- [6] Daniel T Colbert and William H Miller. “A novel discrete variable representation for quantum mechanical reactive scattering via the S-matrix Kohn method”. In: *The Journal of chemical physics* 96.3 (1992), pp. 1982–1991.
- [7] Michael J Davis and Eric J Heller. “Quantum dynamical tunneling in bound states”. In: *The Journal of Chemical Physics* 75.1 (1981), pp. 246–254.
- [8] Koji Hashimoto et al. “Exponential growth of out-of-time-order correlator without chaos: inverted harmonic oscillator”. In: *Journal of High Energy Physics* 2020.11 (2020), pp. 1–25.
- [9] Timothy JH Hele et al. “Boltzmann-conserving classical dynamics in quantum time-correlation functions: “Matsubara dynamics””. In: *The Journal of Chemical Physics* 142.13 (2015), p. 134103.
- [10] Srihari Keshavamurthy and Peter Schlagheck. *Dynamical tunneling: theory and experiment*. CRC Press, 2011.
- [11] Richard B Lehoucq, Danny C Sorensen, and Chao Yang. *ARPACK users’ guide: solution of large-scale eigenvalue problems with implicitly restarted Arnoldi methods*. SIAM, 1998.
- [12] Juan Maldacena, Stephen H Shenker, and Douglas Stanford. “A bound on chaos”. In: *Journal of High Energy Physics* 2016.8 (2016), pp. 1–17.

- [13] John C Mauro, Roger J Loucks, and Jitendra Balakrishnan. “A simplified eigenvector-following technique for locating transition points in an energy landscape”. In: *The Journal of Physical Chemistry A* 109.42 (2005), pp. 9578–9583.
- [14] Jeff Nichols et al. “Walking on potential energy surfaces”. In: *The Journal of chemical physics* 92.1 (1990), pp. 340–346.
- [15] IC Percival. “Regular and irregular spectra”. In: *Journal of Physics B: Atomic and Molecular Physics (1968-1987)* 6.9 (1973), p. L229.
- [16] Ch Skokos and Enrico Gerlach. “Numerical integration of variational equations”. In: *Physical Review E* 82.3 (2010), p. 036704.
- [17] Tianrui Xu, Thomas Scaffidi, and Xiangyu Cao. “Does scrambling equal chaos?” In: *Physical review letters* 124.14 (2020), p. 140602.
